# Supplementary material for: GerontoVis: Data Visualization at the Confluence of Aging
Source: arXiv:2403.13173 ancillary file (2024-03-19)
Supplement: Supplementary file 1 [file expanded_table_1.pdf]

Eurographics Conference on Visualization (EuroVis) 2024
W. Aigner, D. Archambault, and R. Bujack
(Guest Editors)

COMPUTER GRAPHICS *forum*
*Volume 43 (2024), Number 3*

# Supplemental Material:
# *GerontoVis: Data Visualization at the Confluence of Aging*

Zack While[1], R. Jordan Crouser[2], and Ali Sarvghad[1]

[1]Manning College of Information and Computer Sciences, University of Massachusetts, Amherst, USA
[2]Department of Computer Science, Smith College, Northampton, USA

Table 1: Information about the set of 36 papers focusing on older adults and data visualization, including the citation for each paper.

| Domain | # Papers | # Venues | Papers |
|---|---|---|---|
| Health Informatics | 14 | 11 | HLR*13, RLTD13, RCL*14, LRC*14, LRY*15, BDC*16, BCC*16, WPJ18, TRB*18, TYQ18, ATRG*19, TMI*19, FLW23, GCGH23 |
| Computer Science | 11 | 8 | GPBK12, FFD12, LWDT12, DCB15, LTD16, HWC*18, NJLB*19, FWX*23, CHR20, CHLA22, CHD*23 |
| Psychology | 6 | 6 | WM12, LATD14, TRMS17, PCBLP16, CÖ19, MSC*19 |
| Medicine | 5 | 4 | AWR*11, vWAvDJ21, PDSM19, LCC*18, HH14 |

© 2024 The Authors. Computer Graphics Forum published by Eurographics - The European Association for Computer Graphics and John Wiley & Sons Ltd.
This is an open access article under the terms of the Creative Commons Attribution License, which permits use, distribution and reproduction in any medium, provided the original work is properly cited.

## References


[ATRG*19] AHMED R., TOSCOS T., ROHANI GHAHARI R., HOLDEN R. J., MARTIN E., WAGNER S., DALEY C., COUPE A., MIRRO M.: Visualization of Cardiac Implantable Electronic Device Data for Older Adults Using Participatory Design. *Applied Clinical Informatics 10*, 4 (Sept. 2019), 707–718. 1

[AWR*11] ALEXANDER G. L., WAKEFIELD B. J., RANTZ M., SKUBIC M., AUD M. A., ERDELEZ S., GHENAIMI S. A.: Passive sensor technology interface to assess elder activity in independent living. *Nurs Res 60*, 5 (2011), 318–325. 1

[BCC*16] BACKONJA U., CHI N.-C., CHOI Y., HALL A. K., LE T., KANG Y., DEMIRIS G.: Visualization approaches to support healthy aging: a systematic review. *Journal of innovation in health informatics 23*, 3 (2016), 860. 1

[BDC*16] BOCK C., DEMIRIS G., CHOI Y., LE T., THOMPSON H. J., SAMUEL A., HUANG D.: Engaging older adults in the visualization of sensor data facilitated by an open platform for connected devices. *Technology and Health Care 24* (2016), 541–550. 4. URL: https://doi.org/10.3233/THC-161150. 1

[CHD*23] CAJAMARCA G., HERSKOVIC V., DONDIGHUAL S., FUENTES C., VERDEZOTO N.: Understanding how to design health data visualizations for chilean older adults on mobile devices. In *Proceedings of the 2023 ACM Designing Interactive Systems Conference* (2023), pp. 1309–1324. 1

[CHLA22] CAJAMARCA G., HERSKOVIC V., LUCERO A., ALDUNATE A.: A Co-Design Approach to Explore Health Data Representation for Older Adults in Chile and Ecuador. In *Designing Interactive Systems Conference* (New York, NY, USA, 2022), DIS '22, Association for Computing Machinery, p. 1802–1817. URL: https://doi.org/10.1145/3532106.3533558. 1

[CHR20] CAJAMARCA G., HERSKOVIC V., ROSSEL P. O.: Enabling Older Adults' Health Self-Management through Self-Report and Visualization—A Systematic Literature Review. *Sensors 20*, 15 (2020). URL: https://www.mdpi.com/1424-8220/20/15/4348. 1

[CÖ19] CHANG F., ÖSTLUND B.: Perspectives of Older Adults and Informal Caregivers on Information Visualization for Smart Home Monitoring Systems: A Critical Review. In *Proceedings of the 20th Congress of the International Ergonomics Association (IEA 2018)* (Cham, 2019), Bagnara S., Tartaglia R., Albolino S., Alexander T., Fujita Y., (Eds.), Springer International Publishing, pp. 681–690. 1

[DCB15] DOYLE J., CAPRANI N., BOND R.: Older adults' attitudes to self-management of health and wellness through smart home data. In *2015 9th International Conference on Pervasive Computing Technologies for Healthcare (PervasiveHealth)* (2015), pp. 129–136. 1

[FFD12] FAN C., FORLIZZI J., DEY A.: Considerations for Technology That Support Physical Activity by Older Adults. In *Proceedings of the 14th International ACM SIGACCESS Conference on Computers and Accessibility* (New York, NY, USA, 2012), ASSETS '12, Association for Computing Machinery, p. 33–40. URL: https://doi.org/10.1145/2384916.2384923. 1

[FLW23] FELBERBAUM Y., LANIR J., WEISS P. L.: Designing mobile health applications to support walking for older adults. *International Journal of Environmental Research and Public Health 20*, 4 (2023), 3611. 1

[FWX*23] FAN M., WANG Y., XIE Y., LI F. M., CHEN C.: Understanding how older adults comprehend covid-19 interactive visualizations via think-aloud protocol. *International Journal of Human–Computer Interaction 39*, 8 (2023), 1626–1642. 1

[GCGH23] GHORAYEB A., COMBER R., GOOBERMAN-HILL R.: Development of a smart home interface with older adults: Multi-method co-design study. *JMIR Aging 6* (Jun 2023), e44439. URL: https://doi.org/10.2196/44439. 1

[GPBK12] GIUDICE N. A., PALANI H. P., BRENNER E., KRAMER K. M.: Learning Non-Visual Graphical Information Using a Touch-Based Vibro-Audio Interface. In *Proceedings of the 14th International ACM SIGACCESS Conference on Computers and Accessibility* (New York, NY, USA, 2012), ASSETS '12, Association for Computing Machinery, p. 103–110. URL: https://doi.org/10.1145/2384916.2384935. 1

[HH14] HUANG Y.-C., HSU Y.-L.: Social networking-based personal home telehealth system: A pilot study. *Journal of Clinical Gerontology and Geriatrics 5*, 4 (2014), 132–139. URL: https://www.sciencedirect.com/science/article/pii/S2210833514000586. 1

[HLR*13] HUH J., LE T., REEDER B., THOMPSON H. J., DEMIRIS G.: Perspectives on wellness self-monitoring tools for older adults. *Int J Med Inform 82*, 11 (Sept. 2013), 1092–1103. 1

[HWC*18] HARRINGTON C. N., WILCOX L., CONNELLY K., ROGERS W., SANFORD J.: Designing Health and Fitness Apps with Older Adults: Examining the Value of Experience-Based Co-Design. In *Proceedings of the 12th EAI International Conference on Pervasive Computing Technologies for Healthcare* (New York, NY, USA, 2018), PervasiveHealth '18, Association for Computing Machinery, p. 15–24. URL: https://doi.org/10.1145/3240925.3240929. 1

[LATD14] LE T., ARAGON C., THOMPSON H. J., DEMIRIS G.: Elementary graphical perception for older adults: a comparison with the general population. *Perception 43*, 11 (2014), 1249–1260. 1

[LCC*18] LE T., CHI N.-C., CHAUDHURI S., THOMPSON H. J., DEMIRIS G.: Understanding Older Adult Use of Data Visualizations as a Resource for Maintaining Health and Wellness. *Journal of Applied Gerontology 37*, 7 (2018), 922–939. PMID: 27401438. URL: https://doi.org/10.1177/0733464816658751, arXiv:https://doi.org/10.1177/0733464816658751. 1

[LRC*14] LE T., REEDER B., CHUNG J., THOMPSON H., DEMIRIS G.: Design of smart home sensor visualizations for older adults. *Technology and Health Care 22* (2014), 657–666. 4. URL: https://doi.org/10.3233/THC-140839. 1

[LRY*15] LE T., REEDER B., YOO D., AZIZ R., THOMPSON H. J., DEMIRIS G.: An evaluation of wellness assessment visualizations for older adults. *Telemed J E Health 21*, 1 (Jan 2015), 9–15. 1

[LTD16] LE T., THOMPSON H. J., DEMIRIS G.: A Comparison of Health Visualization Evaluation Techniques with Older Adults. *IEEE Computer Graphics and Applications 36*, 4 (2016), 67–77. 1

[LWDT12] LE T., WILAMOWSKA K., DEMIRIS G., THOMPSON H.: Integrated data visualisation: an approach to capture older adults' wellness. *International Journal of Electronic Healthcare 7*, 2 (2012), 89–104. 1

[MSC*19] MOREY S. A., STUCK R. E., CHONG A. W., BARG-WALKOW L. H., MITZNER T. L., ROGERS W. A.: Mobile Health Apps: Improving Usability for Older Adult Users. *Ergonomics in Design 27*, 4 (2019), 4–13. URL: https://doi.org/10.1177/1064804619840731, arXiv:https://doi.org/10.1177/1064804619840731. 1

[NJLB*19] NURGALIEVA L., JARA LACONICH J. J., BAEZ M., CASATI F., MARCHESE M.: A Systematic Literature Review of Research-Derived Touchscreen Design Guidelines for Older Adults. *IEEE Access 7* (2019), 22035–22058. 1

[PCBLP16] PRICE M. M., CRUMLEY-BRANYON J. J., LEIDHEISER W. R., PAK R.: Effects of information visualization on older adults' decision-making performance in a medicare plan selection task: a comparative usability study. *JMIR human factors 3*, 1 (2016), e16. 1

[PDSM19] POIRIER M. W., DECKER C., SPERTUS J. A., MCDOWD J. M.: What eye-tracking methods can reveal about the role of information format in decision-aid processing: an exploratory study. *Patient Education and Counseling 102*, 11 (2019), 1977–1984. URL: https://www.sciencedirect.com/science/article/pii/S0738399118307821. 1

[RCL*14] REEDER B., CHUNG J., LE T., THOMPSON H., DEMIRIS G.:


© 2024 The Authors.
Computer Graphics Forum published by Eurographics and John Wiley & Sons Ltd.

Assessing older adults' perceptions of sensor data and designing visual displays for ambient environments. An exploratory study. *Methods of Information in Medicine 53*, 3 (Apr. 2014), 152–159. 1

[RLTD13] REEDER B., LE T., THOMPSON H. J., DEMIRIS G.: Comparing information needs of health care providers and older adults: findings from a wellness study. *Stud Health Technol Inform 192* (2013), 18–22. 1

[TMI*19] TURCHIOE M. R., MYERS A., ISAAC S., BAIK D., GROSSMAN L. V., ANCKER J. S., CREBER R. M.: A Systematic Review of Patient-Facing Visualizations of Personal Health Data. *Applied Clinical Informatics 10*, 04 (Aug. 2019), 751–770. URL: https://doi.org/10.1055/s-0039-1697592. 1

[TRB*18] THEIS S., RASCHE P. W. V., BRÖHL C., WILLE M., MERTENS A.: Task-Data Taxonomy for Health Data Visualizations: Web-Based Survey With Experts and Older Adults. *JMIR Med Inform 6*, 3 (Jul 2018), e39. 1

[TRMS17] THEIS S., RASCHE P., MERTENS A., SCHLICK C. M.: An Age-Differentiated Perspective on Visualizations of Personal Health Data. In *Advances in Ergonomic Design of Systems, Products and Processes* (Berlin, Heidelberg, 2017), Schlick C. M., Duckwitz S., Flemisch F., Frenz M., Kuz S., Mertens A., Mütze-Niewöhner S., (Eds.), Springer Berlin Heidelberg, pp. 289–308. 1

[TYQ18] TAO D., YUAN J., QU X.: Presenting self-monitoring test results for consumers: the effects of graphical formats and age. *Journal of the American Medical Informatics Association 25*, 8 (2018), 1036–1046. 1

[vWAvDJ21] VAN WEERT J. C., ALBLAS M. C., VAN DIJK L., JANSEN J.: Preference for and understanding of graphs presenting health risk information. The role of age, health literacy, numeracy and graph literacy. *Patient Education and Counseling 104*, 1 (2021), 109–117. 1

[WM12] WHITLOCK L. A., MCLAUGHLIN A. C.: Identifying Usability Problems of Blood Glucose Tracking Apps for Older Adult Users. *Proceedings of the Human Factors and Ergonomics Society Annual Meeting 56*, 1 (2012), 115–119. URL: https://doi.org/10.1177/1071181312561001, arXiv:https://doi.org/10.1177/1071181312561001. 1

[WPJ18] WILDENBOS G. A., PEUTE L., JASPERS M.: Aging barriers influencing mobile health usability for older adults: A literature based framework (MOLD-US). *International Journal of Medical Informatics 114* (Mar. 2018), 66–75. 1

© 2024 The Authors.
Computer Graphics Forum published by Eurographics and John Wiley & Sons Ltd.
